# Supplementary material for: Engineering mixing properties of fluids by spatial modulations
Source: arXiv:2309.14728 ancillary file (2023-09-26)
Supplement: Supplementary file 1 [file supplement.pdf]

# Supplemental Materials: Engineering mixing properties of fluids by spatial modulations

## ENERGY DIAGRAM AND MISCIBILITY

The energetic stability of a globally mixed state can be understood from the energy curve in a diagrammatic manner. Let us consider the globally mixed state with composition $C_0$ that occupies the entire volume $V$, where the composition is defined that the ratio of the number of component 1 atoms to the total number of atoms, $N_1/(N_1+N_2)$. Suppose that this state separates into two phases with composition $C_+(> C_0)$ and $C_-(< C_0)$ that occupies volume $V_+$ and $V_-$, respectively, i.e.,

$$V = V_+ + V_-. \tag{S1}$$

From the assumption $|g_{12} - g| \ll g$, the total density $n_{\rm tot}$ is almost constant. In this case, the conservation of the number of atoms in each component before and after the separation can be expressed as

$$C_0 V = C_+ V_+ + C_- V_-. \tag{S2}$$

The globally mixed state has the energy

$$E_{\rm mix} = V\varepsilon(C_0, n_{\rm tot}), \tag{S3}$$

where $\varepsilon$ is the energy per volume. This energy is marked by the open circle in Fig. S1(a). In the following, $n_{\rm tot}$ is omitted from the arguments of $\varepsilon$, since $n_{\rm tot}$ is kept almost constant. The energy of the separated state is given by $E_{\rm sep} = V_+\varepsilon(C_+) + V_-\varepsilon(C_-)$. Using Eqs. (S1) and (S2), this energy is rewritten as

$$E_{\rm sep} = V\left[\frac{C_+ - C_0}{C_+ - C_-}\varepsilon(C_-) + \frac{C_0 - C_-}{C_+ - C_-}\varepsilon(C_+)\right], \tag{S4}$$

which corresponds to the filled circle in Fig. S1(a), i.e., the intersection point between the vertical line $C = C_0$ and the line connecting the two points $(C_+, \varepsilon(C_+))$ and $(C_-, \varepsilon(C_-))$. Thus, the globally mixed state located within a concave region $(\partial^2\varepsilon/\partial C^2 < 0)$ always has $C_\pm$, such that $E_{\rm sep} < E_{\rm mix}$, and the globally mixed state is energetically unstable against phase separation. Therefore, the inflection point $\partial^2\varepsilon/\partial C^2 = 0$ corresponds to the boundary of the unstable region, which gives the spinodal curve in the phase diagram, as shown in Fig. 4. For the convex region $(\partial^2\varepsilon/\partial C^2 > 0)$, the globally mixed state is stable or metastable. A stable mixed state is given by the tangential point of a line below the energy curve, as shown by the filled circle in Fig. S1(b), because $E_{\rm sep} > E_{\rm mix}$ for any $C_\pm$. This stable region is limited by the tangential points of the lines that touch the edge of the energy curve at $C = 0$ or 1 (dot-dashed line), and therefore, the open circle in Fig. S1(b) gives the binodal curve, as shown in Fig. 4.

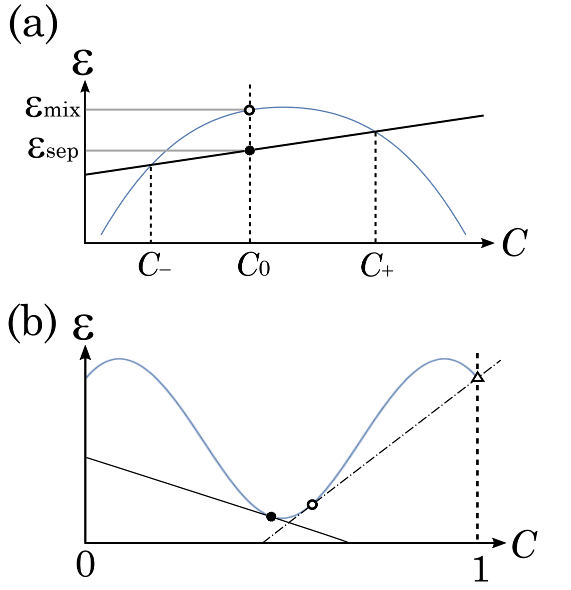


FIG. S1. Diagrammatic representation of the energetic stability of a globally mixed state against phase separation. (a) Energy per volume $\varepsilon$ changes from $\varepsilon_{\rm mix}$ (open circle) to $\varepsilon_{\rm sep}$ (filled circle) if the globally mixed state with composition $C_0$ separates into two phases with composition $C_+$ and $C_-$. (b) Globally mixed state is stable if it corresponds to a tangential point of a line below the energy curve (filled circle). The stable region is limited by the open circle, which is the tangential point of the line through the point $(1, \varepsilon(1))$ (dot-dashed line). When $C$ exceeds the open circle, the globally mixed state separates into the mixed-bubble state (open circle and triangle). Similarly, the lower limit of the stability region is given by the tangential line through $(0, \varepsilon(0))$ (not shown).

## TRAPPED SYSTEM WITH REALISTIC PARAMETERS

We consider an experimental system to observe the phenomena described in the main text. We assume that a two-component Bose-Einstein condensate of $^{23}$Na atoms in the hyperfine states $|F, m_F\rangle = |1, 1\rangle$ (component 1) and $|1, 0\rangle$ (component 2) is confined in a quasi-two-dimensional (2D) circular box trap,

$$V_{\rm trap}(\boldsymbol{r}) = V_0\left(1 + \tanh\frac{r_\perp - R}{w_t}\right) + \frac{1}{2}m\omega_z^2 z^2, \tag{S5}$$

where $V_0$, $R$, and $w_t$ are the height, radius, and rise width of the circular box potential, respectively, $r_\perp = \sqrt{x^2 + y^2}$, and $\omega_z$ is the trap frequency in the $z$ direction. The system is tightly confined in the $z$ direction, and we use the quasi-2D approximation with the effective interaction strength $g_{jj'}^{\rm 2D} = \sqrt{8\pi}a_{jj'}/l_z$ with $l_z = \sqrt{\hbar/(m\omega_z)}$. The $s$-wave scattering lengths are given

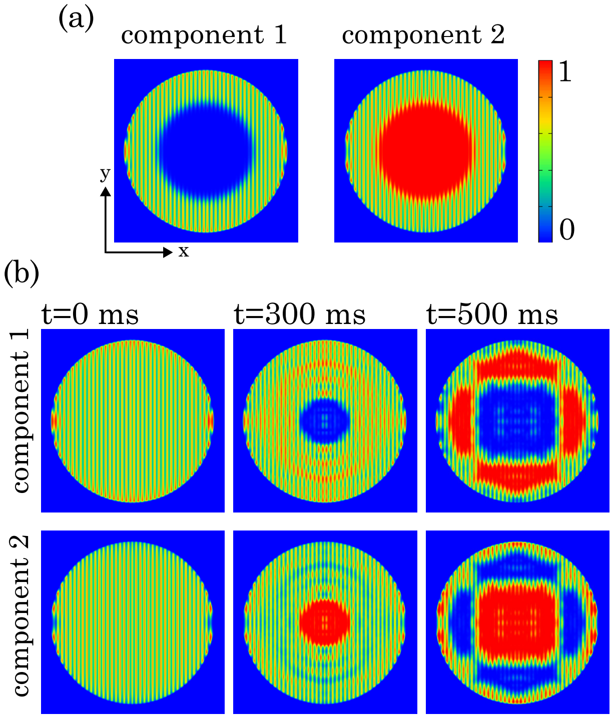


FIG. S2. (a) Mixed-bubble ground state with composition $C = 0.3$ for $U_1 = -U_2 = 1.1\hbar^2 k^2/m$. (b) Dynamics of phase separation via nucleation with $C = 0.5$ for $U_1 = -U_2 = 1.05\hbar^2 k^2/m$. The initial state is the metastable mixed state, and the perturbation potential in Eq. (S6) is given only for the first 100 ms. The size of each panel in (a) and (b) is $220 \times 220$ $\mu$m, and the units of density are $1.6 \times 10^2$ $\mu\text{m}^{-2}$.

by $a_{11} = a_{12} = 54.54a_0$ and $a_{22} = 52.66a_0$, where $a_0$ is the Bohr radius [1]. These scattering lengths satisfy the immiscible condition $a_{12}^2 > a_{11}a_{22}$ in a homogeneous system. The periodic potential $V_j(\boldsymbol{r}) = U_j \cos^2(kx)$ is generated by the interference of two laser beams, where the wave number $k$ can be controlled by the angle between the laser beams. Here we take the parameters $2\pi/k = 10$ $\mu$m, $R = 100$ $\mu$m, $w_t = 1$ $\mu$m, $\omega_z/(2\pi) = 4$ kHz, and $V_0 = 100\hbar^2 k^2/m$. In this case, $l_z \simeq 0.3$ $\mu$m, and the 2D approximation can safely be used. The total number of condensate atoms is $N = 5 \times 10^6$, which gives the peak density $\simeq 3 \times 10^{14}$ $\text{cm}^{-3}$. The spin-exchanging collision can be suppressed by a strong magnetic field [2].

Figure S2 shows the results obtained by numerically solving the Gross-Pitaevskii equation. The mixed-bubble ground state with composition $C = N_1/N = 0.3$ for $U_1 = -U_2 = 1.1\hbar^2 k^2/m$ is shown in Fig. S2(a), where the mixed phase coexists with the phase occupied by component 2. Figure S2(b) shows the dynamics of phase separation via nucleation with $C = 0.5$ for $U_1 = -U_2 = 1.05\hbar^2 k^2/m$. The initial state is the metastable mixed state, as shown in the leftmost panels. A local perturbation potential,

$$V_p(\boldsymbol{r}) = V_{p0} \exp[-(r_\perp/w_p)^2], \tag{S6}$$

is added from $t = 0$ to $t = 100$ ms, where $V_{p0} = 4\hbar^2 k^2/m$ and $w_p = 2$ $\mu$m. The phase separation is triggered by the perturbation potential and extends over the entire system at $t = 500$ ms.

[1] S. Knoop, T. Schuster, R. Scelle, A. Trautmann, J. Appmeier, and M. K. Oberthaler, Feshbach spectroscopy and analysis of the interaction potentials of ultracold sodium, Phys. Rev. A **83**, 042704 (2011).

[2] H.-J. Miesner, D. M. Stamper-Kurn, J. Stenger, S. Inouye, A. P. Chikkatur, and W. Ketterle, Observation of metastable states in spinor Bose-Einstein condensates, Phys. Rev. Lett. **82**, 2228 (1999).
